# Supplementary material for: HyperG: Hypergraph-Enhanced LLMs for Structured Knowledge
Source: arXiv:2502.18125 source file (2025-02-25)
Supplement: Supplementary file 1 [file 7_appendix.tex]

\section{Prompt Templates}\label{apdx:prompt}

\begin{figure}[H]
    \centering
  \begin{minipage}[t]{\linewidth} %
    \subfigure[An example prompt for the TFV task.]{
        \label{fig:barchart1}
        \includegraphics[width=\linewidth]{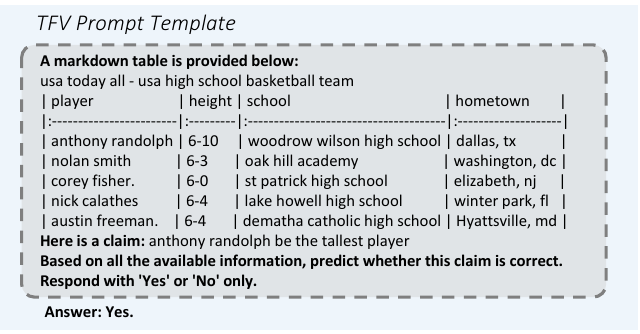}
    }  
  \end{minipage}
  \begin{minipage}[t]{\linewidth} %
    \subfigure[An example prompt for the TQA task.]{
        \label{fig:barchart2}
        \includegraphics[width=\linewidth]{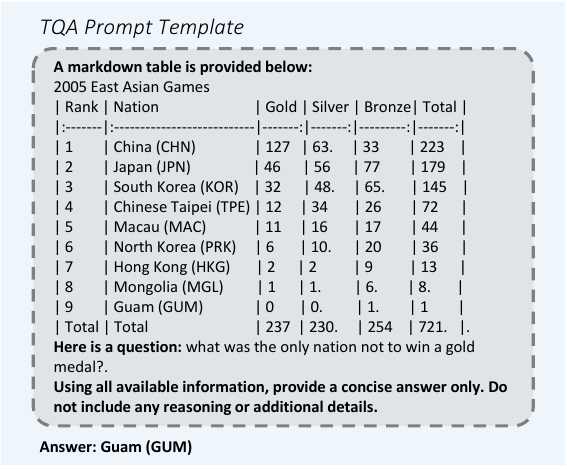}
    }  
  \end{minipage}
  \caption{Examples of the prompts used in the TFV and TQA experiments in this paper.}
    \label{fig:prompts}
\end{figure}

\section{Case Study}\label{apdx:case}

% \begin{figure}[H]
%     \centering
%     \includegraphics[width=1.03\columnwidth]{figures/case_study2.pdf}
%     \caption{LLM-augmented row descriptions and visualization of the average weights across 12 attention heads between cell nodes and their corresponding row hyperedges for a table with missing values. Note that some rows are omitted for simplicity. The average weight for all the edges in this hypergraph is 0.27.}
%     \label{fig:case2}
% \end{figure}

% \begin{figure}[t!]
%     \centering
%     \includegraphics[width=1.03\columnwidth]{figures/case_study.pdf}
%     \caption{Visualization of the weights between cell nodes and corresponding column hyperedges and the table hyperedge.}
%     \label{fig:case}
% \end{figure}

This randomly selected table presents records from the 1961 Victorian Football League (VFL) season, an Australian football league. The inquiry related to this table claims that the Junction Oval venue had the highest crowd attendance. To verify this claim, LLMs need to focus on the ``Crowd'' column and the venue name "Junction Oval" in the 5th row, as highlighted in Figure \ref{fig:case}. As illustrated in Section \ref{sec:SHC}, each cell in the table is considered a node, while the columns, rows, and the entire table are treated as hyperedges in \name. The bottom two subfigures illustrate the average weights across the 12 attention heads between each cell node and the corresponding column hyperedges (left), and that between nodes and the table hyperedge (right). It can be observed that: 1) The attention weights for both the connections between cell nodes and column hyperedges, as well as the table hyperedge, focus on the highlighted part and the ``Date'' column. In addition, since the inquiry pertains to the \textit{highest} crowd participation, the first and the last row, which have obvious lower participation values, receive lower attention weights, specifically 0.33 and 0.24, respectively. 2) The connections with the table hyperedge exhibit more smoothed attentions compared to the column hyperedges. This is because the table hyperedge is initialized using the caption embedding, which is inherently related to all the cells in the table.
